# Supplementary material for: Predicting Hypoxia in Brain Tumors from Multiparametric MRI
Source: arXiv:2401.14171 source file (2024-01-25)
Supplement: Supplementary file 1 [file Supplementary.tex]

\section{Supplementary}
\subsection{Pre-processing strategies of k-space}
\label{section:prepro}

Pre-processing is a crucial step in deep learning. It refers to the transformation and manipulation of input data before it is fed into the model. The goal of k-space pre-processing is to boost the model's performance helping with an estimation of the missed lines. We used two basic pre-processing types of the under-sampling data in order to fill the zeros values either with the surround values (neighbor level is 2), called mean strategy or take the benefits of the read-conjugate symmetry of the k-space, called symmetry strategy (see more details in the following section \ref{section:preproCS}). In severe or extreme under-sampling the two above pre-processing strategies can only fill partly of the missed lines, for this reason, we also apply a combination of conjugate symmetry and mean strategies, called combination strategy. Firstly, we applied the conjugate symmetry strategy, and the rest of the missed lines were filled by the mean strategy.
In summary, in this project we are trying the following pre-processing strategies: 1) without any pre-processing, 2) mean, 3) conjugate symmetry, and 4) combination of mean and conjugate symmetry. 

\subsubsection{Conjugate symmetry}
\label{section:preproCS}
In MRI (Magnetic Resonance Imaging), the signal detected by the receiver coil is represented in the frequency domain as a spectrum of complex numbers, with each number representing a different frequency component of the signal. The complex spectrum has a property called "conjugate symmetry", which means that the frequency components above and below the center frequency are complex conjugates of each other []. Conjugate symmetry in MRI is a result of the Fourier transform [], which is used to convert the time-domain signal to the frequency domain. The Fourier transform of a real-valued signal produces a complex spectrum with conjugate symmetry. 

Conjugate symmetry is important in MRI data processing, as it can be used to reduce the amount of data that needs to be stored and processed []. By taking advantage of the conjugate symmetry, the data can be "folded" or "mirrored" along the center frequency, effectively reducing the amount of data by a factor of two. In addition, many MRI reconstruction algorithms use the conjugate symmetry property to improve the image quality and reduce artifacts. By exploiting the symmetry of the data, these algorithms can reconstruct images with higher spatial resolution and better signal-to-noise ratio [].

\begin{figure}[ht!]
  \centering
  \begin{minipage}{.6\textwidth}
    \begin{subfigure}{\textwidth}
      \centering
      \subcaptionOverlay{\includegraphics[width=\textwidth]{Images/conjugateSummetry.png}}
    \end{subfigure}
  \end{minipage}
  \begin{minipage}{.2\textwidth}
    \begin{subfigure}{\textwidth}
      \centering
      \subcaptionOverlay{\includegraphics[width=\textwidth]{Images/maskGR78faster.jpg}}
    \end{subfigure}
    \begin{subfigure}{\textwidth}
      \centering
      \subcaptionOverlay{\includegraphics[width=\textwidth]{Images/maskGR78fasterCS.jpg}}
    \end{subfigure}
  \end{minipage}
  \caption{Conjugate (Hermitian) symmetry of k-space. Mirror image locations across the origin of k-space have real components of the same sign but imaginary components of the opposite sign.}
% https://mriquestions.com/partial-fourier.html
    \label{fig:methodsCS} 
\end{figure}

Read-conjugate symmetry is a partial Fourier technique where data in one-half of k-space is used to synthesize/predict data in the other half. The direction of symmetry is in the readout (frequency-encode direction). Mirror image locations across the origin of k-space have real components of the same sign but imaginary components of the opposite sign []. For example, conjugate symmetry applies to pairs of points (like P and Q in figure \ref{fig:methodsCS}) that are located diagonally from each other across the origin of k-space. If the data at P is the complex number [a+bi], the data at Q is immediately known to be P's complex conjugate, [a-bi]. 
% https://mriquestions.com/partial-fourier.html

\begin{figure}[ht!]
  \centering
  \includegraphics[width=0.9\textwidth]{Images/ImportancePreProImage.png}
  \caption{Images of different pre-processing strategies}
    \label{fig:resultsprepro} 
\end{figure}

Figure \ref{fig:resultsprepro} displays the impact of the k-space pre-processing. The first, second, third, and fourth columns represent the ground truth, the under-sampling image, the output of the K-net model, and the output of the I-net model, respectively. The first, second, third, and fourth lines show  the result with the following pre-processing strategies: without any pre-processing, mean, conjugate symmetry, and combination, respectively. In the following table (ref) the SSIM and MSE matrices are reported for the four different pre-processing strategies. However, the results are quite similar 

\begin{table}[ht!]
    \begin{center}
        \begin{tabular}{l|cccc}
            \textit{SSMI} & 60\%  & 70\%  & 80\%   \\
            \hline
            \hline
            Without & 0,89 $\pm$ 0.02 & 0,82 $\pm$ 0.04 & 0,85 $\pm$ 0.03  \\
            Mean  & 0,89 $\pm$ 0.02 & 0,83 $\pm$ 0.04 & 0,85 $\pm$ 0.03  \\
            Conjugate symmetry  & 0,89 $\pm$ 0.03 & 0,82 $\pm$ 0.04 & 0,85 $\pm$ 0.03  \\
            Combination & 0,87 $\pm$ 0.03 & 0,83 $\pm$ 0.04 & 0,85 $\pm$ 0.03  \\
            \textit{FSIM} &   &   &   \\
            \hline
            \hline
            Without & 0,986 $\pm$ 0.001 & 0,978 $\pm$ 0.002 & 0,960 $\pm$ 0.004  \\
            Mean  & 0,986 $\pm$ 0.002 & 0,978 $\pm$ 0.002 & 0,960 $\pm$ 0.004  \\
            Conjugate symmetry  & 0,985 $\pm$ 0.001 & 0,978 $\pm$ 0.002 & 0,956 $\pm$ 0.004  \\
            Combination & 0,986 $\pm$ 0.002 & 0,979 $\pm$ 0.002 & 0,957 $\pm$ 0.004  \\
            \textit{PSNR} &   &   &   \\
            \hline
            \hline
            Without & 30.55 $\pm$ 1.60 & 29.10 $\pm$ 1.43 & 28.07 $\pm$ 1.88 \\
            Mean  &  30.76 $\pm$ 1.59 & 29.32 $\pm$ 1.49 & 28.85 $\pm$ 1.98 \\
            Conjugate symmetry  &  30.87 $\pm$ 1.58 & 29.41 $\pm$ 1.47 & 28.06 $\pm$ 1.86 \\
            Combination &  30.76 $\pm$ 1.61 & 29.61 $\pm$ 1.49 & 27.80 $\pm$ 1.93 \\
            \textit{MSE} $(10^{-3})$ &   &   &   \\
            \hline
            \hline
            Without & 0.946 $\pm$ 0.388 &  1.130 $\pm$ 0.458 &  1.718 $\pm$ 0.812  \\
            Mean  & 0.900 $\pm$ 0.359 &  1.235 $\pm$ 0.412 &  1.833 $\pm$ 0.962  \\
            Conjugate symmetry  & 0.872 $\pm$ 0.312 &  1.206 $\pm$ 0.396 &  1.726 $\pm$ 0.846  \\
            Combination & 0.895 $\pm$ 0.319 &  1.155 $\pm$ 0.372 &  1.846 $\pm$ 0.953  \\
        \end{tabular}
    \end{center}
    \label{tab:resultspreproT1} 
    \caption{Table: impact of the pre-processing}
\end{table}

\begin{figure}[ht!]
  \centering
  \includegraphics[width=0.9\textwidth]{Images/ImportancePreProplots.png}
  \caption{metrics plots of Different levels of US degradation and pre-processing strategy - No need it ???}
    \label{fig:resultspreprodegradationplots} 
\end{figure}

\begin{table*}[t]
    \label{tab:resultspreproT} 
    \caption{Table: impact of the different Under-sampling masks and levels reference metrics }
     \begin{tabular}{l||ccc|ccc}
            \textbf{ US masks}   & \multicolumn{3}{c}{Reference Metrics}    & \multicolumn{3}{c}{Reference free Metrics}   \\
              &  SSIM  &  SSIMf  & PSNR & SNR  & Contrast & Sharpness \\
            \hline
            \hline
            Ground Truth &  -   & -  & -  & 15.249 $\pm$ 2.170  & 0.671 $\pm$ 0.141 & 0.879 $\pm$ 0.039 \\
            \hline
            \hline
             Uniform & 0.750 $\pm$ 0.043 & 0.977 $\pm$ 0.006 & 78.112 $\pm$ 1.434 & 44.159 $\pm$ 0.000 & 0.701 $\pm$ 0.000  & 0.784 $\pm$ 0.000\\
             Random & 0.747 $\pm$ 0.043 & 0.977 $\pm$ 0.007 & 77.742 $\pm$ 1.445 & 40.989 $\pm$ 0.000 & 0.699 $\pm$ 0.000 & 0.775 $\pm$ 0.000 \\
             Gradient &\textbf{0.760 $\pm$ 0.043} & \textbf{0.979 $\pm$ 0.006} & \textbf{78.447 $\pm$ 1.457} & 51.656 $\pm$ 0.000 & 0.708 $\pm$ 0.000  & \textbf{0.798 $\pm$ 0.000} \\
             Mixed & 0.669 $\pm$ 0.048 & 0.978 $\pm$ 0.006 & 77.514 $\pm$ 1.212 & \textbf{53.758 $\pm$ 0.000} & \textbf{0.725 $\pm$ 0.000}  & 0.794 $\pm$ 0.000\\
             
            \\
            \textbf{ US Acceleration}   & \multicolumn{3}{c}{}    & \multicolumn{3}{c}{ }   \\
              &   &   &  &  & & \\
            \hline
            \hline
            3.3x & 0.760 $\pm$ 0.043 & 0.979 $\pm$ 0.006 & 78.447 $\pm$ 1.457 & 51.656 $\pm$ 0.000 & 0.708 $\pm$ 0.000  & 0.798 $\pm$ 0.000 \\
            5x & 0.609 $\pm$ 0.048 & 0.971 $\pm$ 0.008 & 76.496 $\pm$ 1.175 & 77.125 $\pm$ 11.824 & 0.735 $\pm$ 0.154 & 0.739 $\pm$ 0.059 \\
            10x & 0.682 $\pm$ 0.047 & 0.962 $\pm$ 0.011 & 74.934 $\pm$ 1.798 & 107.222 $\pm$ 16.006 & 0.746 $\pm$ 0.148 & 0.630 $\pm$ 0.067 \\

            \\
            \textbf{PP strategies}   & \multicolumn{3}{c}{}    & \multicolumn{3}{c}{ }   \\
              &   &   &  &  & & \\
            \hline
            \hline
            Without  & 0.760 $\pm$ 0.043 & 0.979 $\pm$ 0.006 & 78.447 $\pm$ 1.457 & 51.656 $\pm$ 0.000 & 0.708 $\pm$ 0.000  & 0.798 $\pm$ 0.000 \\
            5x & 0.609 $\pm$ 0.048 & 0.971 $\pm$ 0.008 & 76.496 $\pm$ 1.175 & 77.125 $\pm$ 11.824 & 0.735 $\pm$ 0.154 & 0.739 $\pm$ 0.059 \\
            10x & 0.682 $\pm$ 0.047 & 0.962 $\pm$ 0.011 & 74.934 $\pm$ 1.798 & 107.222 $\pm$ 16.006 & 0.746 $\pm$ 0.148 & 0.630 $\pm$ 0.067 \\
            10x & 0.682 $\pm$ 0.047 & 0.962 $\pm$ 0.011 & 74.934 $\pm$ 1.798 & 107.222 $\pm$ 16.006 & 0.746 $\pm$ 0.148 & 0.630 $\pm$ 0.067 \\

        \end{tabular}
\end{table*}
